# Supplementary material for: OpenForge: Probabilistic Metadata Integration
Source: arXiv:2412.09788 source file (2024-12-13)
Supplement: Supplementary file 1 [file 09_supplementary.tex]

\clearpage
\section{Supplementary Material}

\subsection{Benchmark Samples}\label{subsec:benchmark_samples}

  Table~\ref{tab:arts_samples},~\ref{tab:sotab_samples},~\ref{tab:icpsr_samples}, and~\ref{tab:artsmr_samples} give samples of relation instances from ARTS, SOTAB, ICPSR, and ARTS-MR benchmarks, respectively.

  \begin{table}[h]
    \centering
    \caption{Relation instance samples from ARTS benchmark.}
    \label{tab:arts_samples}
    \resizebox{\columnwidth}{!}{%
    \begin{tabular}{cc}
      \toprule
      Concept Pairs & Relation \\ \midrule
      number of incidents, identification number & Null \\
      zip code, name of street & Null \\
      percentage of graduates, percentage of teachers & Null \\
      geographic longitude coordinates, geographical coordinates & Null \\
      average number, number of clients & Null \\
      name of organization, organization name & Equivalent \\
      percentage of students, percentage of student population & Equivalent \\
      percentage of teachers, percent of teachers & \multicolumn{1}{l}{Equivalent} \\
      geographic coordinate, geographical location coordinates & Equivalent \\
      longitude coordinate, geographic longitude coordinates & Equivalent \\ \bottomrule
    \end{tabular}}%
  \end{table}

  \begin{table}[h]
    \centering
    \caption{Relation instance samples from SOTAB benchmark.}
    \label{tab:sotab_samples}
    \resizebox{0.85\columnwidth}{!}{%
    \begin{tabular}{cc}
      \toprule
      Concept Pairs & Relation \\ \hline
      music album name, musical artist & Null \\
      album, creative work series & Null \\
      price, rating & Null \\
      url, brand & Null \\
      sports team, sports event & Null \\
      address locality, locality & Equivalence \\
      music album name, album & Equivalence \\
      music artist, musical artist & Equivalence \\
      tv episode name, television episode & Equivalence \\
      book name, book & Equivalence \\ \hline
    \end{tabular}}%
  \end{table}

  \begin{table}[h]
    \centering
    \caption{Relation instance samples from ICPSR benchmark.}
    \label{tab:icpsr_samples}
    \resizebox{\columnwidth}{!}{%
    \begin{tabular}{cc}
      \toprule
      Concept Pairs & Relation \\ \midrule
      psychological evaluation, educational policy & Null \\
      economic reform, financial assets & Null \\
      executive power, Nixon Administration (1969-1974) & Null \\
      property crime statistics, international crime statistics & Null \\
      health care services, family relationships & Null \\
      offenses, vandalism & Hypernymy \\
      economic indicators, durable goods & Hypernymy \\
      durable goods, automobiles & \multicolumn{1}{l}{Hypernymy} \\
      criminal justice programs, inmate release plans & Hypernymy \\
      health care services, mental health services & Hypernymy \\ \bottomrule
    \end{tabular}%
    }
  \end{table}

  \begin{table}[hb]
    \centering
    \caption{Relation instance samples from ARTS-MR benchmark.}
    \label{tab:artsmr_samples}
    \resizebox{0.95\columnwidth}{!}{%
    \begin{tabular}{cc}
    \toprule
    Concept Pairs & Relation \\ \midrule
    page number, building number & Null \\
    effective date, completion date & Null \\
    \begin{tabular}[c]{@{}c@{}}borough block lot number,\\ name of nyc borough\end{tabular} & Null \\
    \begin{tabular}[c]{@{}c@{}}community board identification number,\\ census tract identification number\end{tabular} & Null \\
    \begin{tabular}[c]{@{}c@{}}numeric code for state senate district,\\ type of code used for student discharge or transfer\end{tabular} & Null \\
    name, name of recipient & Hypernymy \\
    \begin{tabular}[c]{@{}c@{}}latin name,\\ latin name of tree species\end{tabular} & \multicolumn{1}{l}{Hypernymy} \\
    effective date, effective date of permit & Hypernymy \\
    \begin{tabular}[c]{@{}c@{}}type of complaint,\\ type of complaint made to 311\end{tabular} & Hypernymy \\
    \begin{tabular}[c]{@{}c@{}}page number,\\ page number of expense report\end{tabular} & Hypernymy \\
    \begin{tabular}[c]{@{}c@{}}nyc borough name,\\ name of new york city borough\end{tabular} & Equivalence \\
    \begin{tabular}[c]{@{}c@{}}date when the data was collected,\\ the date on which the data was collected\end{tabular} & Equivalence \\
    census tract id number, census tract number & Equivalence \\
    \begin{tabular}[c]{@{}c@{}}zip code of business location,\\ zip code of business\end{tabular} & Equivalence \\
    \begin{tabular}[c]{@{}c@{}}number of students in grades 9 through 12,\\ number of students enrolled in grades 9 to 12\end{tabular} & Equivalence \\ \bottomrule
    \end{tabular}%
    }
  \end{table}

\clearpage
\subsection{GPT Prompts}\label{subsec:gpt_prompts}
  We use the following prompts including task descriptions and few-shot learning for GPT models in the experiments of ICPSR and ARTS-MR benchmarks. We omit prompts for ARTS and SOTAB benchmarks as they are mostly identical to the one of ICPSR benchmark except for the different relation type for classification.

\noindent """

Your task is to determine whether two concepts are hypernymy, which means that first concept has broader meaning than the second one. Return your final result in the following JSON format : {"answer": <yes or no>}.

For example:

Input:

Concept 1: organizations

Concept 2: student organizations

Output:

{"answer": "yes"}

Input:

Concept 1: reform

Concept 2: transition economies

Output:

{"answer": "yes"}

Input:

Concept 1: Obama Administration (2009-  )

Concept 2: space technology

Output:
{"answer": "no"}

Input:

Concept 1: First Amendment

Concept 2: freedom of the press

Output:
{"answer": "yes"}

Input:

Concept 1: social stratification

Concept 2: communications systems

Output:

{"answer": "no"}

Input:

Concept 1: recidivists

Concept 2: presidential administrations

Output:

{"answer": "no"}

Input:

Concept 1: patient care

Concept 2: post-hospitalization care

Output:

{"answer": "yes"}

Input:

Concept 1: school vandalism

Concept 2: participation

Output:

{"answer": "no"}

Input:

Concept 1: economic indicators

Concept 2: electronics

Output:

{"answer": "yes"}

Input:

Concept 1: consolidated metropolitan statistical areas

Concept 2: health care facilities

Output:

{"answer": "no"}

Now, for the following concept pairs, please determine if they are hypernymy. Return your final result in the following JSON format : {"answer": <yes or no>}.

Input:

Concept 1: human settlements

Concept 2: administrative divisions

Output:

\noindent"""

\noindent"""

Your task is to determine whether two concepts are (1) hypernymy, which means that first concept has broader meaning than the second one, (2) equivalent, which means that two concepts are considered semantically equivalent, or (3) NULL, which means that there is no relation between the two concepts.  Return your final result in the following JSON format : {"answer": <"hypernymy" or "equivalent" or "NULL">}.

Input:

Concept 1: name

Concept 2: name of new york city borough

Output:

{"answer": "hypernymy"}

Input:

Concept 1: numeric code

Concept 2: page number of expense report

Output:

{"answer": "NULL"}

Input:

Concept 1: payment type

Concept 2: the payment type used for the trip

Output:

{"answer": "hypernymy"}

Input:

Concept 1: name

Concept 2: latin name of tree species

Output:

{"answer": "hypernymy"}

Input:

Concept 1: name of the ferry terminal where the complaint / request occurred ( if applicable )

Concept 2: name of the ferry terminal where the complaint or request was made

Output:

{"answer": "equivalent"}

Input:

Concept 1: borough block lot number

Concept 2: name of the ferry terminal where the complaint or request was made

Output:

{"answer": "NULL"}

Input:

Concept 1: numeric code

Concept 2: numeric code for state senate district

Output:

{"answer": "hypernymy"}

Input:

Concept 1: census tract id number

Concept 2: census tract identification number

Output:

{"answer": "equivalent"}

Input:

Concept 1: community board number in nyc

Concept 2: name of the ferry terminal where the complaint / request occurred ( if applicable )

Output:

{"answer": "NULL"}

Input:

Concept 1: name of the ferry terminal where the complaint / request occurred ( if applicable )

Concept 2: name of the ferry terminal involved in the complaint or issue

Output:

{"answer": "equivalent"}

Now, for the following concept pairs, please determine if they are hypernymy, equivalent or NULL relation. Return your final result in the following JSON format : {"answer": <"hypernymy" or "equivalent" or "NULL">}.

Input:

Concept 1: code

Concept 2: code for the location where the building is located

Output:

\noindent"""
